# Supplementary material for: Subtle Signals: Video-based Detection of Infant Non-nutritive Sucking as a Neurodevelopmental Cue
Source: arXiv:2310.16138 source file (2023-10-24)
Supplement: Supplementary file 1 [file supplementary.tex]

\newcommand{\supp}{
\newpage
\onecolumn
\newcommand{\beginsupplement}{%
        \setcounter{table}{0}
        \setcounter{equation}{0}
        \renewcommand{\theequation}{S\arabic{equation}}
        \setcounter{section}{0}
        \renewcommand{\thetable}{S\arabic{table}}%
        \setcounter{figure}{0}
        \renewcommand{\thefigure}{S\arabic{figure}}%
}
%\maketitle
\newcommand{\independent}{\protect\mathpalette{\protect\independenT}{\perp}}
\def\independenT##1##2{\mathrel{\rlap{$##1##2$}\mkern2mu{##1##2}}}
\renewcommand\thesection{\Alph{section}}
\beginsupplement
\newcommand{\MYhref}[3][blue]{\href{##2}{\color{##1}{##3}}}

\section{Supplementary Material} 

% \tblcompare
